# Supplementary material for: Signed Graph Autoencoder for Explainable and Polarization-Aware Network Embeddings
Source: arXiv:2409.10452 source file (2025-03-10)
Supplement: Supplementary file 1 [file 6-appendix.tex]

\clearpage
\section{Supplementary}
\begin{table*}[ht]\caption{List of notations.}
\begin{center}% used the environment to augment the vertical space
% between the caption and the table
\begin{tabular}{r c p{10cm} }
\toprule
$n$ & $\triangleq$ & Total number of nodes\\
$k$ & $\triangleq$ & Number of communities\\
$c_i$ & $\triangleq$ & Community assignment for node $i$\\
$\mathbf{c}$ & $\triangleq$ & Community membership array\\  
$p_{in}^{+}$ & $\triangleq$ & Probability of a positive edge within the same community\\ 
$p_{in}^{-}$ & $\triangleq$ & Probability of a negative edge within the same community\\ 
$p_{out}^{+}$ & $\triangleq$ & Probability of a positive edge between different communities\\
$p_{out}^{-}$ & $\triangleq$ & Probability of a negative edge between different communities\\
\bottomrule
\end{tabular}
\end{center}
\label{tab:TableOfNotationForMyResearch}
\end{table*}

\subsection*{Details of the GNN-based Encoder}

For each encoder we use two GCN layer with $64$ input and output hidden dimensions for each. For each network node we use as feature the $32$ first eigenvectors of the signed Normalized Laplacian of the network. For all MLPs we use $64$ hidden dimensions.

\subsection*{Algorithm for Signed network generation}
We next provide the algorithm to generate a signed network showcasing \textsc{2-level Polarization}.

\begin{algorithm}[H]
\caption{Signed Network Generation for \textsc{2-level Polarized} Networks}
\begin{algorithmic}[1]
    \State Initialize twp empty graphs $G_{pos}$ and $G_{neg}$ with the $n$ same nodes.
    \State Assign each node $i$ to a positive community for $G_{pos}$ via $c^{pos}_i$ and a negative community for $G_{neg}$ via $c^{neg}_i$ based on the community membership arrays $\mathbf{c^{pos}}$,$\mathbf{c^{neg}}$.
    \For {$c_i$ in $\{c^{pos}_i,c^{neg}_i\}$}
    \For{each pair of nodes $(i, j)$ with $i < j$}
        \If{$c_i = c_j$}
            \State Draw $r \sim \text{Uniform}(0, 1)$.
            \If{$r < p_{in}^{+}$}
                \State Add an edge $(i, j)$ with weight $+1$.
            \ElsIf{$r < p_{in}^{+} + p_{in}^{-}$}
                \State Add an edge $(i, j)$ with weight $-1$.
            \EndIf
        \Else
            \State Draw $r \sim \text{Uniform}(0, 1)$.
            \If{$r < p_{out}^{+}$}
                \State Add an edge $(i, j)$ with weight $+1$.
            \ElsIf{$r < p_{out}^{+} + p_{out}^{-}$}
                \State Add an edge $(i, j)$ with weight $-1$.
            \EndIf
        \EndIf
    \EndFor
    \State Return the graph $G=G_{pos}-G_{neg}$.
\end{algorithmic}
\end{algorithm}

\subsection{Additional Details}
